# Supplementary material for: Robust RL with LLM-Driven Data Synthesis and Policy Adaptation for Autonomous Driving
Source: arXiv:2410.12568 source file (2024-10-20)
Supplement: Supplementary file 1 [file appendix_jx.tex]

\clearpage
\section{Appendix}

Schema:
\begin{enumerate}
    \item Distil LLM knowledge to RL agent, then fine-tune the RL agent for driving tasks. (Must show that compare to vanilla RL supervised training, the LLM knowledge improves the performance)
    \item Fine-tune the RL agent for driving tasks, then distill LLM knowledge to RL. This investigate if LLM knowledge can improve the decision making of RL agent (but likely not, prove the 1)
    \item Jointly fine-tune the RL agent with distillation LLM as a regularization term. This combine 1 and 2.
\end{enumerate}

Robustness:
\begin{enumerate}
    \item Given the RL agent, improve the robustness via adversarial training.
    \item Given the LLM, improve the robustness before distilling into RL agent. (Need to verify if this approach improves the robustness of RL agent as well when fine-tuning with driving tasks).
    \item Jointly perform 1 and 2. (If 2 is actually useful)
\end{enumerate}

\begin{section}
    LLM sampled data is effective and valuable, it can support the offline RL training. 
\end{section}
